# Supplementary material for: Digital 3D Smocking Design
Source: arXiv:2309.07201 source file (2023-09-13)
Supplement: Supplementary file 1 [file appendix_fsp.tex]

\section{Regular Full Smocking Pattern}\label{appendix:formulation:regular_pattern}
As discussed in Definition~\ref{defi:regular-pattern}, we mainly consider solving the smocking design from a \emph{regular} pattern. Here we discuss the undesirable effects that an irregular pattern might cause.

\setlength{\columnsep}{3pt}%
\setlength{\intextsep}{1pt}%
\begin{wrapfigure}{r}{0.5\linewidth}
\centering
\begin{overpic}[trim=0cm 0cm 0cm 0cm,clip,width=1\linewidth,grid=false]{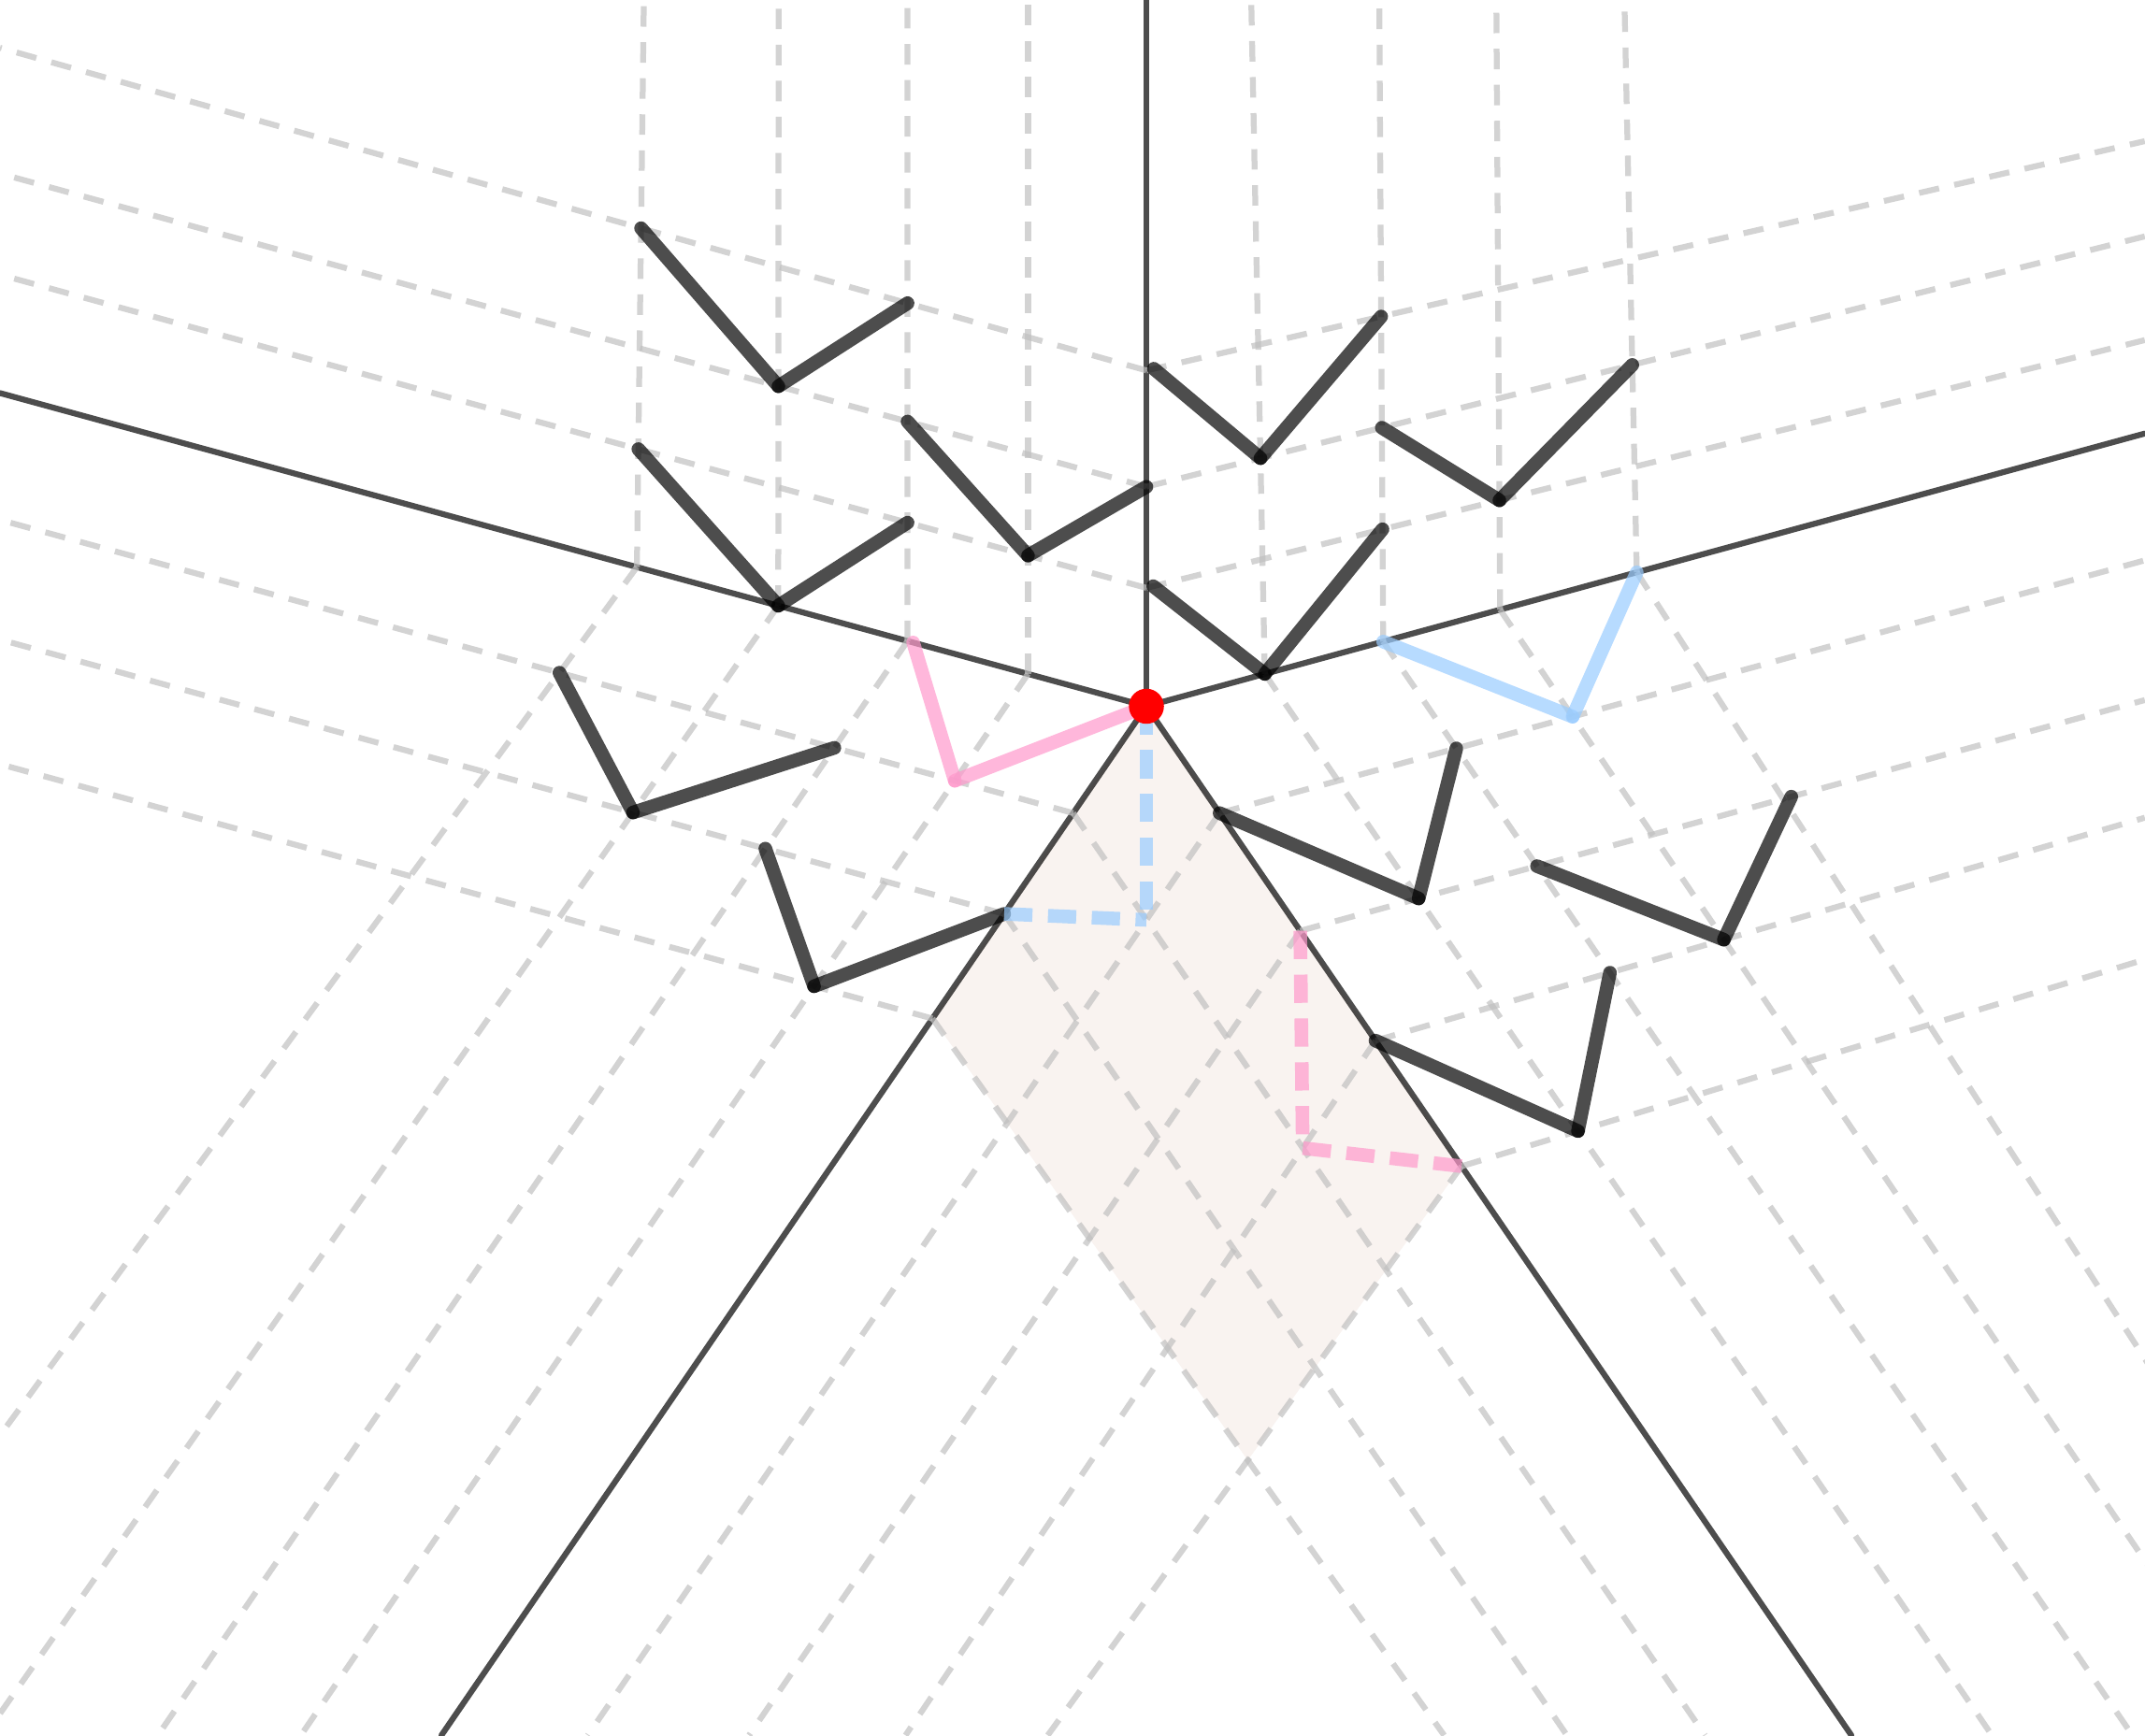}
\end{overpic}
\end{wrapfigure}
\paragraph{Singularity.} 
In this work, we do not consider the case when there exists singularity in the grid of the smocking pattern. See the inset figure for an example, where we highlight the grid singularity by red dot.
We can see that tiling the unit smocking pattern in the highlighted region is ambiguous. 
Specifically, we will get the \emph{blue} dashed stitching line if we follow the pattern in the \emph{right} region. If we keep this stitching line, it will merge two stitching lines on the left region together.
On the other hand, if we follow the pattern in the \emph{left} region, we will get the \emph{pink} dashed stitching line, which will make the smocking texture irregular when combined with the stitching lines on the left region. 
To alleviate such irregular textures, we considered using radial grid to tile the pattern in cyclic order without tiling around the singularity region (see Fig.~\ref{fig:res:radial_grids}).
We leave this for future work of designing reasonable tiling to handle grids with general singularities. 

\setlength{\columnsep}{3pt}%
\setlength{\intextsep}{1pt}%
\begin{wrapfigure}{r}{0.5\linewidth}
\centering
\begin{overpic}[trim=0cm 0cm 0cm 0cm,clip,width=1\linewidth,grid=false]{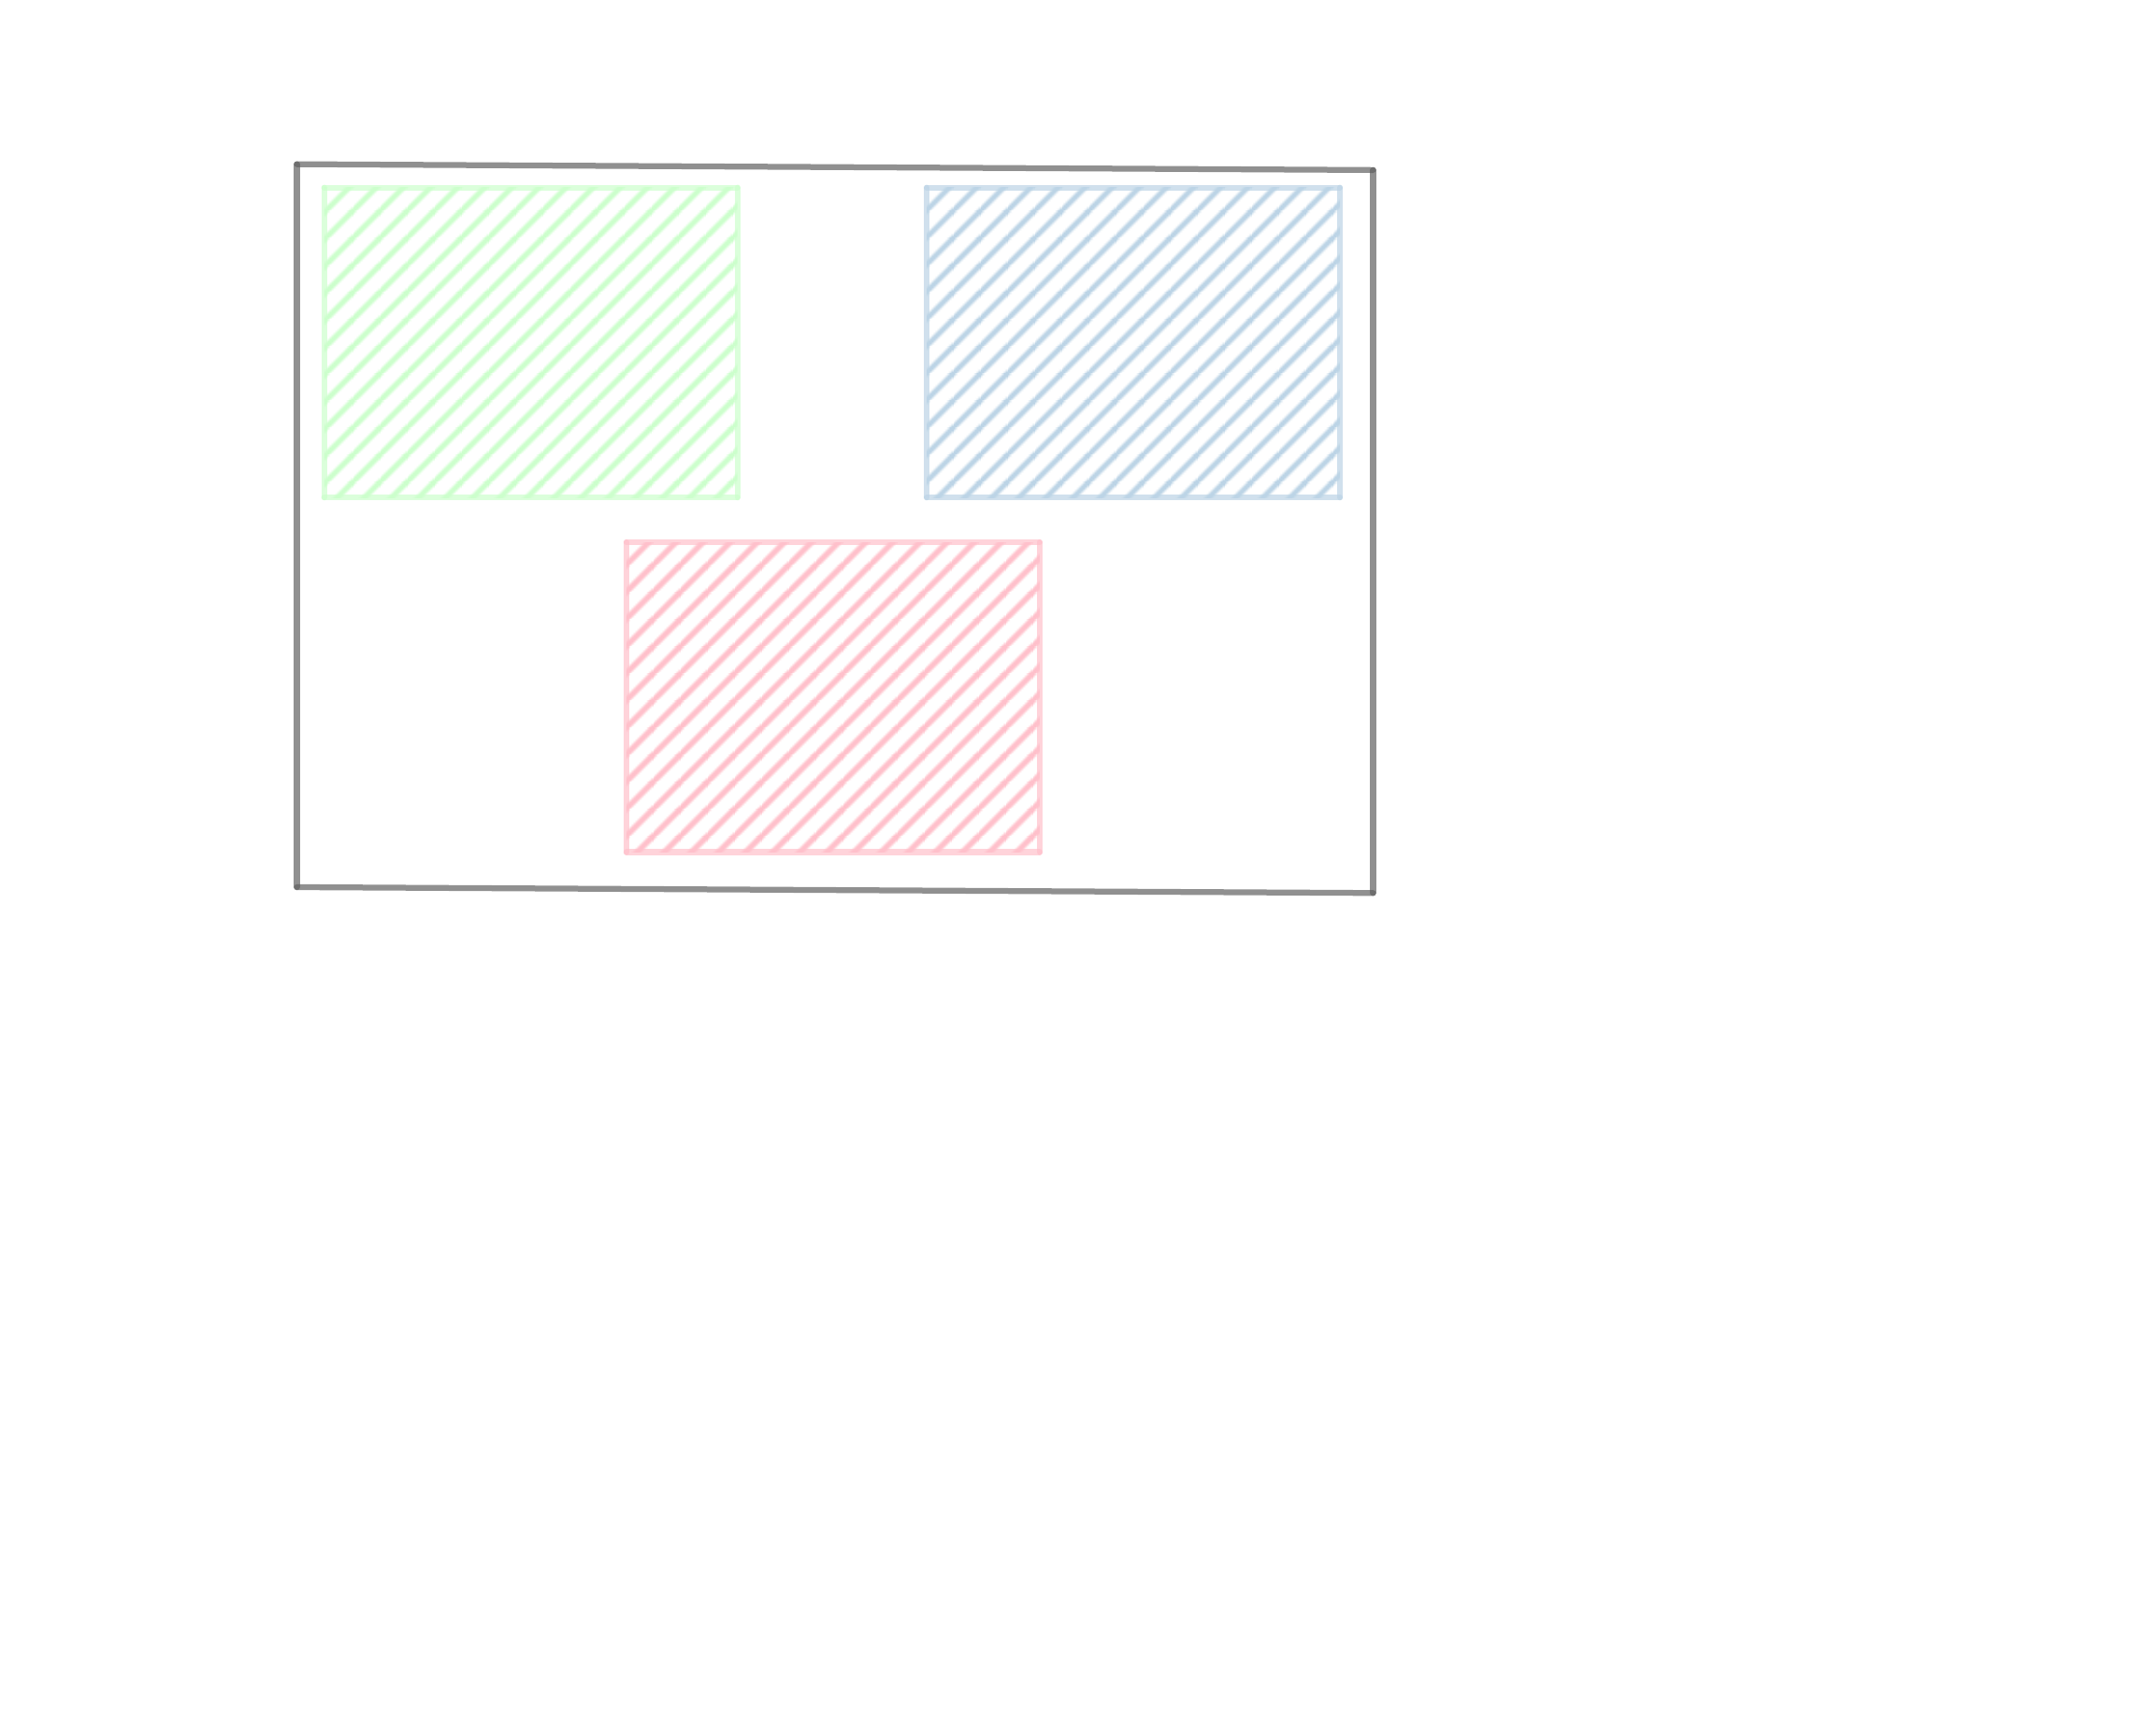}
\end{overpic}
\end{wrapfigure}
\paragraph{Irregular Tiling.} 
We also assume the unit smocking pattern are \emph{regularly} tiled on a fabric to get the full pattern for smocking, leading to a fully connected underlay/pleat graph. See the inset figure as a counterexample, where some unit pattern is tiled inside the green/blue/pink regions only, and the rest region is plain.
During smocking, the space between the green and blue region cannot be preserved, since smocking the pink region makes the inbetween space shrinked, which invalidates the equality constraints for the underlay graph established between the green and blue region. 
In this case, we need to modify our algorithm to handle the underlay graph between different regions. Or alternatively, we can first solve for smocking design in each region independently and then integrate them together.
Note that, our method can handle irregular grids with different grid sizes or deformed shape as discussed in the main text. The irregularity we are discussing here is about tiling the unit pattern across an arbitrary grid, which is not necessarily a regular grid with unit spacing.
